# Supplementary material for: Optimal grouping of arbitrary diagrammatic expansions via analytic pole structure
Source: arXiv:1911.11129 ancillary file (2019-11-25)
Supplement: Supplementary file 1 [file Supplemental_Material.pdf]

# Supplemental Material: Optimal grouping of arbitrary diagrammatic expansions via analytic pole structure

Amir Taheridehkordi,[1] S. H. Curnoe,[1] and J. P. F. LeBlanc[1,*]

[1] *Department of Physics and Physical Oceanography, Memorial University of Newfoundland, St. John's, Newfoundland & Labrador A1B 3X7, Canada*

(Dated: November 25, 2019)

## I. EXAMPLE: ARRAY REPRESENTATION OF DIAGRAMS

Essential to our method is to represent Feynman diagrams in an array form. In this section we provide an example to elucidate the array representation of the Hubbard self-energy diagrams. We consider a third order diagram shown in Figure S1. We first assign a frequency-momenta label to the diagram in order to construct the usual symbolic representation. We note that there is a double pole with respect to $i\nu_1$ while other poles are simple. The temporal part of the diagram is then given by (up to a convergence factor)

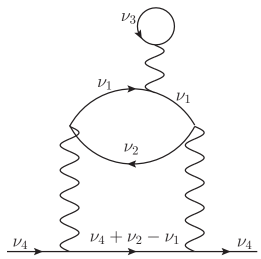


Figure S1. A third order diagram in the perturbative expansion of the Hubbard self-energy. We assign a frequency-momenta label to the diagram.

$$I^{(3)} = \frac{1}{\beta^3}\sum_{\nu_1,\nu_2,\nu_3}\mathcal{I}^{(3)} = \frac{1}{\beta^3}\sum_{\nu_1,\nu_2,\nu_3}\mathcal{G}_0^1(i\nu_1)\mathcal{G}_0^2(i\nu_1)\mathcal{G}_0^3(i\nu_2)\mathcal{G}_0^4(i\nu_3)\mathcal{G}_0^5(i\nu_4+i\nu_2-i\nu_1)$$
$$= \frac{1}{\beta^3}\sum_{\nu_1,\nu_2,\nu_3}\frac{1}{i\nu_1-e_1}\frac{1}{i\nu_1-e_1}\frac{1}{i\nu_2-e_2}\frac{1}{i\nu_3-e_3}\frac{1}{i\nu_4+i\nu_2-i\nu_1-e_4}. \quad (1)$$

Each Green's function in the summand includes two parts: energies and linear combination of the frequencies, which can be extracted from the set of $\alpha$ values obtained from the labeling. We first represent the energies in the array form:

$$\begin{aligned} e_1 = \epsilon(\mathbf{k}_1) &\to (1,0,0,0,0),\\ e_2 = \epsilon(\mathbf{k}_2) &\to (0,1,0,0,0),\\ e_3 = \epsilon(\mathbf{k}_3) &\to (0,0,1,0,0),\\ e_4 = \epsilon(\mathbf{k}_4+\mathbf{k}_2-\mathbf{k}_1) &\to (0,0,0,1,0). \end{aligned} \quad (2)$$

The second part of the $j$th entry is the array representation of the frequency part of the $j$th Green's function, which is given by

$$\begin{aligned} i\nu_1 &\to (1,0,0,0),\\ i\nu_2 &\to (0,1,0,0),\\ i\nu_3 &\to (0,0,1,0),\\ i\nu_4+i\nu_2-i\nu_1 &\to (-1,1,0,1). \end{aligned} \quad (3)$$

We finally achieve the array representation of the summand:

$$\mathcal{I}^{(3)} \to \Big[[(1,0,0,0,0),(1,0,0,0)];[(1,0,0,0,0),(1,0,0,0)];[(0,1,0,0,0),(0,1,0,0)];[(0,0,1,0,0),(0,0,1,0)];$$
$$[(0,0,0,1,0),(-1,1,0,1)]\Big]. \quad (4)$$

Since there is a double pole the first two entries of the array (4) are identical, and we get four distinct energies

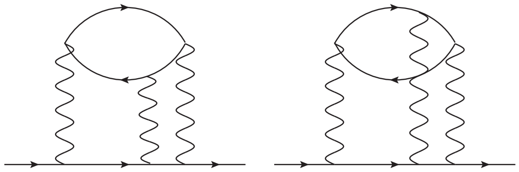

Figure S2. Two topologically distinct third order Hubbard self-energy diagrams, which we denote by $\Sigma_1^{(3)}$ and $\Sigma_2^{(3)}$, respectively. Since these two diagrams are almost isomorphic one expects them to be either equal or cancelling at half-filling.

and frequencies.

We remind that in the AMI full analytic result the dispersion and frequency parts in each term are linear combinations of the initial arrays in Eq. (2) and Eq. (3), which can be evaluated exactly (up to machine precision) in numeric momenta integration procedures.

## II. EXAMPLE: APPLICATION OF GIT

In this section we aim to explicitly demonstrate how one can apply GIT procedure to determine whether two given diagrams are equal/cancelling or not at half-filling. We consider two third order diagrams, shown in Figure S2, arising from the perturbative expansion of self-energy function of the Hubbard model. The first step is to assign a conserving frequency-momenta label to each diagram. Finding the labels enables us to construct mathematical expressions of the diagrams:

$$\Sigma_1^{(3)} = \frac{U^3}{\beta^3}\sum_{\{\mathbf{k}\}}\sum_{\{\nu\}} \frac{1}{i\nu_1-\epsilon(\mathbf{k}_1)}\frac{1}{i\nu_2-\epsilon(\mathbf{k}_2)}\frac{1}{i\nu_3-\epsilon(\mathbf{k}_3)}\frac{1}{i\nu_4-i\nu_1+i\nu_2-\epsilon(\mathbf{k}_4-\mathbf{k}_1+\mathbf{k}_2)}\times \frac{1}{i\nu_4-i\nu_3+i\nu_2-\epsilon(\mathbf{k}_4-\mathbf{k}_3+\mathbf{k}_2)} = \frac{U^3}{\beta^3}\sum_{\{\mathbf{k}\}}\sum_{\{\nu\}} L_1^{(3)}, \tag{5}$$

$$\Sigma_2^{(3)} = \frac{U^3}{\beta^3}\sum_{\{\mathbf{k}\}}\sum_{\{\nu\}} \frac{1}{i\nu_1-\epsilon(\mathbf{k}_1)}\frac{1}{i\nu_2-\epsilon(\mathbf{k}_2)}\frac{1}{i\nu_3-\epsilon(\mathbf{k}_3)}\frac{1}{i\nu_4+i\nu_1-i\nu_2-\epsilon(\mathbf{k}_4+\mathbf{k}_1-\mathbf{k}_2)}\times \frac{1}{i\nu_4+i\nu_3-i\nu_2-\epsilon(\mathbf{k}_4-\mathbf{k}_2+\mathbf{k}_3)} = \frac{U^3}{\beta^3}\sum_{\{\mathbf{k}\}}\sum_{\{\nu\}} L_2^{(3)}, \tag{6}$$

where $L_i^{(3)}$ is the symbolic representation of the $\Sigma_i^{(3)}$ integrand. One notes that in this representation diagrams have the same pole-ID. Starting with $L_1^{(3)}$, our task is to find a combination of GIT transformations $\mathcal{T}$ under which $\Sigma_1^{(3)}$ is invariant and $\mathcal{T} : L_1^{(3)} = \pm L_2^{(3)}$. As the first transformation, we apply $\mathcal{T}_2$ on all the internal variables of $\Sigma_1^{(3)}$, i.e.:

$$\begin{aligned}\mathcal{T}_2 :&(i\nu_1,\mathbf{k}_1) \to (-i\nu_1,-\mathbf{k}_1),\\ &(i\nu_2,\mathbf{k}_2) \to (-i\nu_2,-\mathbf{k}_2),\\ &(i\nu_3,\mathbf{k}_3) \to (-i\nu_3,-\mathbf{k}_3).\end{aligned} \tag{7}$$

We then have

$$\Sigma_1^{(3)} = \frac{U^3}{\beta^3}\sum_{\{\mathbf{k}\}}\sum_{\{\nu\}} \frac{1}{-i\nu_1-\epsilon(\mathbf{k}_1)}\frac{1}{-i\nu_2-\epsilon(\mathbf{k}_2)}\frac{1}{-i\nu_3-\epsilon(\mathbf{k}_3)}\frac{1}{i\nu_4+i\nu_1-i\nu_2-\epsilon(\mathbf{k}_4+\mathbf{k}_1-\mathbf{k}_2)}\times \frac{1}{i\nu_4+i\nu_3-i\nu_2-\epsilon(\mathbf{k}_4+\mathbf{k}_3-\mathbf{k}_2)}. \tag{8}$$

Next we impose:

$$\begin{aligned}\mathcal{T}_3 :&\mathbf{k}_1 \to \mathbf{k}_1+(\pi,\pi),\\ &\mathbf{k}_2 \to \mathbf{k}_2+(\pi,\pi),\\ &\mathbf{k}_3 \to \mathbf{k}_3+(\pi,\pi),\end{aligned} \tag{9}$$

which leads to

$$\Sigma_1^{(3)} = \frac{U^3}{\beta^3} \sum_{\{\mathbf{k}\}} \sum_{\{\nu\}} \frac{1}{-i\nu_1 + \epsilon(\mathbf{k}_1)} \frac{1}{-i\nu_2 + \epsilon(\mathbf{k}_2)} \frac{1}{-i\nu_3 + \epsilon(\mathbf{k}_3)} \frac{1}{i\nu_4 + i\nu_1 - i\nu_2 - \epsilon(\mathbf{k}_4 + \mathbf{k}_1 - \mathbf{k}_2)} \times \frac{1}{i\nu_4 + i\nu_3 - i\nu_2 - \epsilon(\mathbf{k}_4 + \mathbf{k}_3 - \mathbf{k}_2)}. \tag{10}$$

Comparing Eq.(10) and Eq. (6) we find out

$$\Sigma_2^{(3)} = -\Sigma_1^{(3)}, \tag{11}$$

i.e., the two third order diagrams in the diagrammatic expansion of the Hubbard self-energy with nearest neighbor hopping are cancelling at half-filling. In addition, GIT returns a transformation that maps $\mathcal{T} : L_1^{(3)} \to -L_2^{(3)}$:

$$\mathcal{T} = \mathcal{T}_3 \mathcal{T}_2. \tag{12}$$

## III. TRUNCATION ERROR

We truncate the self-energy series expansion at a specific order $m_c$, we therefore need to estimate the error due to the truncation. For a series $\sum_{n=1}^{\infty} b_n$, the absolute truncation error is given by

$$e = \sum_{n=m_c+1}^{\infty} b_n. \tag{13}$$

Since in practice one could only evaluate finite terms of the expansion we have to estimate the truncation error under specific circumstances. We consider two different scenarios and present estimates for the upper bound of the truncation error.

### A. Estimation of Truncation Error for Alternating Sign Series

An alternating sign series is a series where the terms alternate between positive and negative, i.e., $\sum_{n=1}^{\infty} b_n$ is alternating sign if $b_{n+1}/b_n < 0$. An alternating sign series $\sum_{n=1}^{\infty} b_n$ is convergent if it satisfies two criteria:

1. Its $n$th term converges to zero:

$$\lim_{n\to\infty} b_n = 0. \tag{14}$$

2. The absolute values of its terms are decreasing:

$$|\frac{b_{n+1}}{b_n}| < 1. \tag{15}$$

Under these conditions the upper bound of the absolute truncation error is estimated by

$$e \leq |b_{m_c+1}|, \tag{16}$$

where $m_c$ is the truncation order.

### B. Estimation of Truncation Error for Non-Alternating Sign Series

We start with Eq. (13) to determine an upper bound for the absolute error:

$$e \leq \sum_{n=m_c+1}^{\infty} |b_n| = |b_{m_c+1}| \left(1 + \sum_{n=1}^{\infty} \left| \frac{b_{m_c+n+1}}{b_{m_c+1}} \right| \right). \tag{17}$$

We now assume that the series $\sum_{n=1}^{\infty} b_n$ is not alternating sign, however, the sequence $\{r_n = |b_{n+1}/b_n|\}$ is decreasing and $r_n < 1$ for $n > m_c$. We then have

$$e \leq |b_{m_c+1}| \left[1 + \sum_{n=1}^{\infty} \left| \frac{b_{m_c+2}}{b_{m_c+1}} \right|^n \right]. \tag{18}$$

Calculating the power series in the bracket, we finally obtain an upper limit for the error:

$$e \leq \frac{|b_{m_c+1}|}{1 - \frac{|b_{m_c+2}|}{|b_{m_c+1}|}}. \tag{19}$$

* jleblanc@mun.ca
